# Supplementary material for: A Multi-Layout Design for Immersive Visualization of Network Data
Source: arXiv:2112.10272 source file (2023-01-26)
Supplement: Supplementary file 1 [file usecases.tex]

% \documentclass[../supplemental.tex]{subfiles}

% \begin{document}
\section{Use Cases}
We present use cases for each of our views based on one of our datasets~\cite{celegansneural}. The data represents the nervous system of a C. Elegans worm encoded as a network. Each node represents a neuron. Edges indicate functional connections between those neurons (synapses and gap junctions).

In these examples, we show the workflow of finding neurons with strong and diverse inter-community connectivity using our suite's layouts. For a visual tour through this workflow, please refer to the supplemental video.

\subsection{Overview Layout}
% At a glance: Can be used for orientation
In the overview layout, the user identifies the overall structure of the neural network at a glance. Color coding of communities allows her to quickly identify 13 major functional groups of the nervous system. She is also able to see that some groups are more densely connected than others.

\subsection{Spherical Layout}
%  Identify community structures, size, the connection between communities, etc.
% Not well suited for detailed analysis but gives a good impression of the relationship between communities
After gaining a first impression of the data, the user decides to expand the layout into the spherical view. The edge bundling and wide spreading of communities make it easier to see broad connection patterns in the neural network. The user identifies several candidate groups that stand out due to their strong bundles of edges. These groups might play a central role in the worm's nervous system.

\subsection{Floating Community Layout}
% Well suited to identify how a single community relates to the whole of the network
The floating layout allows the user to inspect candidate communities in more detail. The rendering will emphasize inter-community edges that leave a selected community. In this view, it is easy to discern neurons with strong external connectivity from those that are mainly connected to others in the same group. By expanding multiple communities simultaneously, the user can find nodes that share a connection, make judgements about the interplay of neuron clusters, and identify communities that connect to a large number of other clusters.

\subsection{Projected Community Layout}
% Good to identify the structure of a single community. The focus should def be on just this single community and its intra-community edges.
% Less suited to judge connections to other parts of the network.
Once the user finds such a diversely connected community, she activates the projected layout for that community to spread it across the floor. In this view, the user will have enough space to closely inspect all the nodes one by one. She identifies several nodes that have strong inter-community connectivity and notes down their names.

% \biblio
% \end{document}
